# Supplementary material for: To BEE or not to BEE: Estimating more than Entropy with Biased Entropy Estimators
Source: arXiv:2501.11395 source file (2025-01-20)
Supplement: Supplementary file 1 [file appendix.tex]

\clearpage

\begin{table}[h!]
    \centering
    \begin{adjustbox}{width=1\textwidth}
    \begin{tabular}{ c c }
    \includegraphics[width=0.5\textwidth, height=43mm]{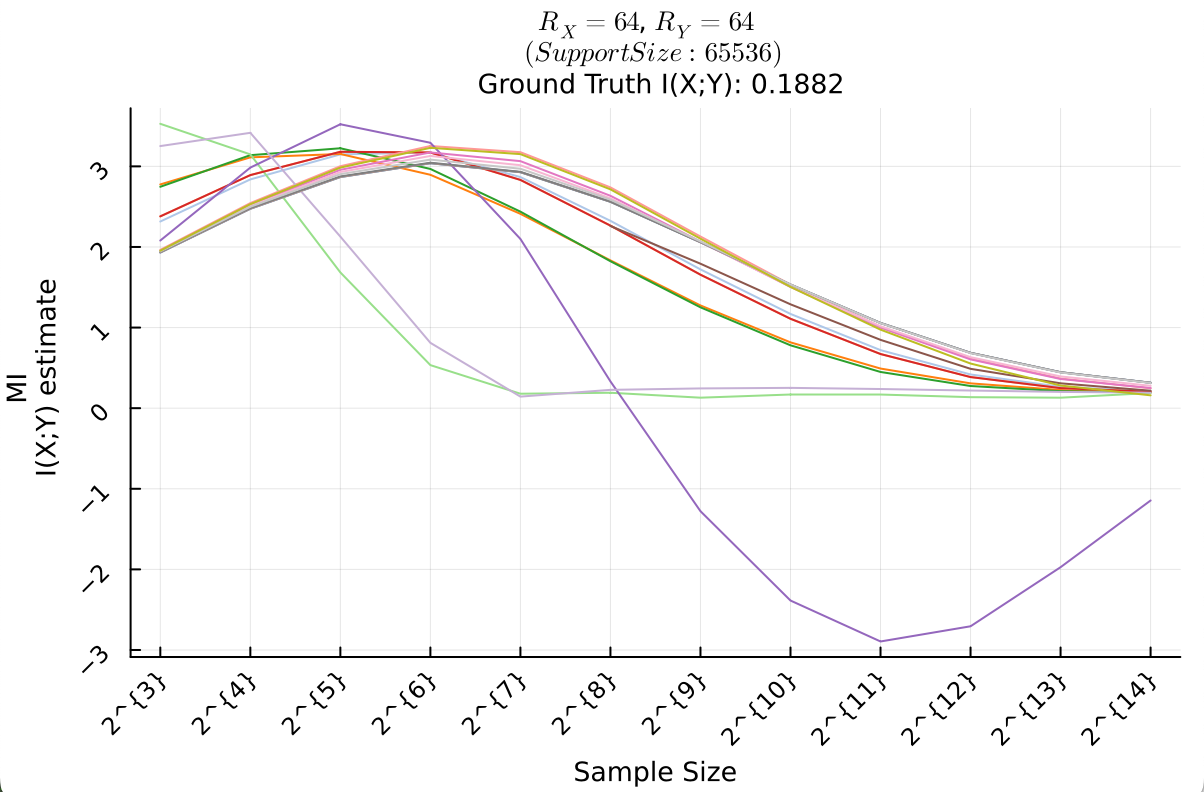} & 
    \includegraphics[width=0.5\textwidth, height=43mm]{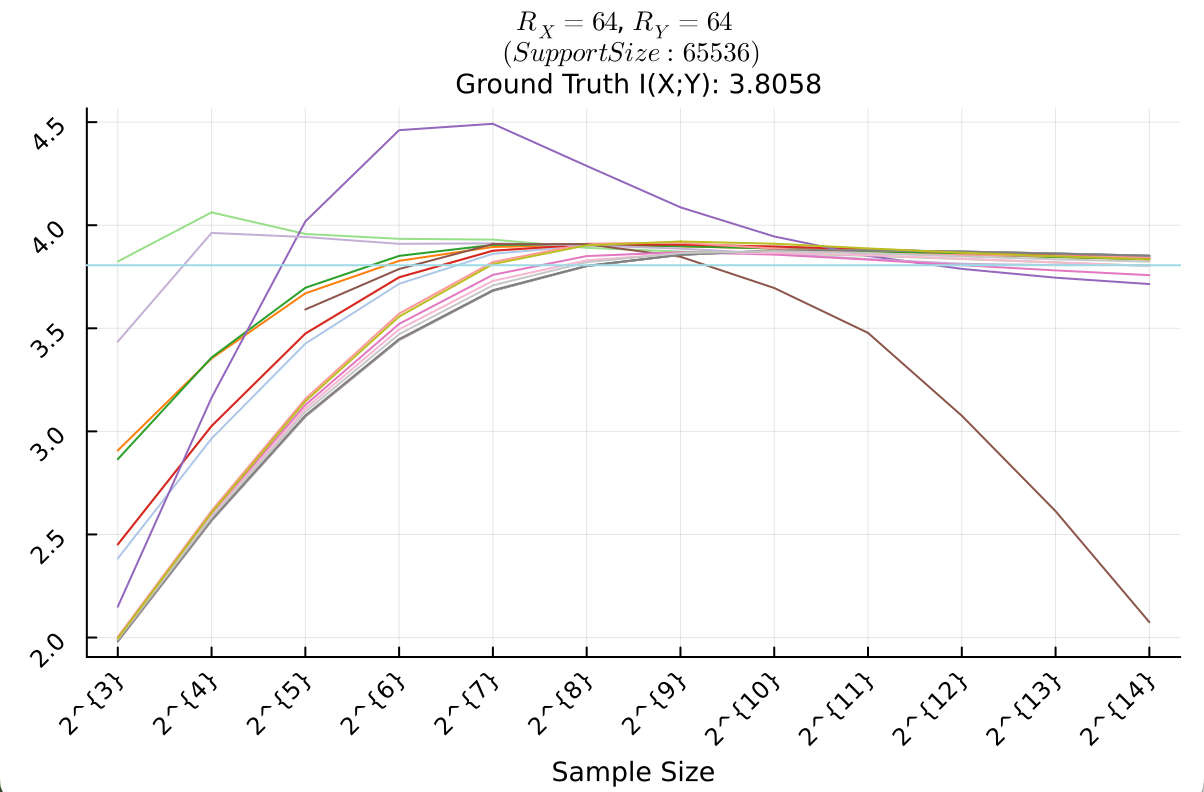} \\
    \arrayrulecolor{lightgray}\hline
    \includegraphics[width=0.5\textwidth, height=43mm]{images/CMI/CMI_min_64.png}  & \includegraphics[width=0.5\textwidth, height=43mm]{images/CMI/CMI_max_64.png} \\
    \end{tabular}
    \end{adjustbox}
    \caption{MI estimations ($1^{st}$ row), CMI estimations ($2^{nd}$ row). GT  $\sim$ 0 ($1^{st}$ column), GT  $\sim$ max ($2^{nd}$ column).\\ Input Space 16384.}
    \label{tab:mi_cmi_estimation_min_max_16384}
\end{table}
